# Supplementary material for: The Power of Synchronisation: Formal Analysis of Power Consumption in Networks of Pulse-Coupled Oscillators
Source: arXiv:1709.04385 source file (2017-10-24)
Supplement: Supplementary file 1 [file appendix.tex]

\newpage
\onecolumn
\section*{Appendix}

\begin{equation}
	f(\theta_0, \ldots, \theta_{N-1}) =
		\sqrt
		{
			\left(
				\frac
					{\sum_{i=0}^{N-1} \cos \theta_i}
					{N}
			\right)^2
			+
			\left(
				\frac
					{\sum_{i=0}^{N-1} \sin \theta_i}
					{N}
			\right)^2					
		} 
		\label{eq:f}
\end{equation}
Observing that
\begin{equation}
	\left( \sum_{i=0}^{k-1} x_i \right)^2 =
%	\left( \sum_{i=0}^{k-1} x_i \right) \left( \sum_{j=0}^{k-1} x_j \right) =
%	\sum_{i=0}^{k-1} x_i \left(x_i + \sum_{j \ne i} x_j \right) = 
	\sum_{i=0}^{k-1} {x_i}^2 + 2 \sum_{i=0}^{k-1} \sum_{j=0}^{i-1} x_j x_i
\end{equation}
we can rewrite Eq.~\ref{eq:f} as
\begin{IEEEeqnarray}{lll}
	\nonumber
	f(\theta_0, \ldots, \theta_{N-1})
		& = &
		\sqrt
		{
				\frac{1}{N^2}
				\left(
					\displaystyle\sum_{i=0}^{N-1} \cos^2 \theta_i + 2 \sum_{i=0}^{N-1} \sum_{j=0}^{i-1} \cos \theta_i \cos \theta_j +
					\displaystyle\sum_{i=0}^{N-1} \sin^2 \theta_i + 2 \sum_{i=0}^{N-1} \sum_{j=0}^{i-1} \sin \theta_i \sin \theta_j
				\right)
		} \\
		\nonumber
		& = &
		\frac{1}{N}
		\sqrt
		{
				N + 
					2 \sum_{i=0}^{N-1} \sum_{j=0}^{i-1} 
					\left(									
						\cos \theta_i \cos \theta_j + \sin \theta_i \sin \theta_j
					\right) 
		} \\
		\nonumber
		& = &
		\frac{1}{N}
		\sqrt
		{
				N + 2 \sum_{i=0}^{N-1} \sum_{j=0}^{i-1}  \cos (\theta_i - \theta_j ) .
		} \\
\end{IEEEeqnarray}
The partial derivatives of $f$ with respect to $\theta_k$ for $0 \le k < N$ are then given by
\begin{IEEEeqnarray}{lll}
	\frac{\partial f}{\partial \theta_k}
	\left(
		\frac{1}{N}
		\sqrt
		{
				N + 2 \sum_{i=0}^{N-1} \sum_{j=0}^{i-1}  \cos (\theta_i - \theta_j )
		}
	\right) \\
	\nonumber
	= 
	\frac
		{1}
		{2 N \sqrt{N + 2 \displaystyle\sum_{i=0}^{N-1} \sum_{j=0}^{i-1}  \cos (\theta_i - \theta_j)}}
	\frac
		{\partial}{\partial \theta_k} 
	\left(		
		N + 2 \sum_{i=0}^{N-1} \sum_{j=0}^{i-1}  \cos (\theta_i - \theta_j )
	\right) \\
	\nonumber
	= 
	\frac
		{1}
		{2 N \sqrt{N + 2 \displaystyle\sum_{i=0}^{N-1} \sum_{j=0}^{i-1}  \cos (\theta_i - \theta_j)}}
			2 \sum_{i\ne k} \sin (\theta_i - \theta_k) \\
	\nonumber
	\label{eq:fderiv}
\end{IEEEeqnarray}
To find the critical points of $f$ we require $\frac{\partial f}{\partial \theta_k}$ to
be $0$ for all $0 \le k < N$. Since one or both factors of Eq.~\ref{eq:fderiv} must
therefore be equal to $0$, and the fractional factor has no solution for $0$, we can
conclude that it must be the case that
$\sum_{i \ne k} \sin (\theta_i - \theta_k)= 0$
for $0 \le k < N$, and therefore that
$\sum_{k=0}^{N-1} \sum_{i \ne k} \sin (\theta_i - \theta_k) = 0$.
Furthermore, we can see that
$\sum_{k=0}^{N-1} \sum_{i \ne k} \sin (\theta_i - \theta_k) =
\sum_{k=0}^{N-2} \sum_{i=k+1}^{N-1} \sin (\theta_i - \theta_k)  - \sin(\theta_k - \theta_i)= 0$.
